# Supplementary material for: A Complex KBQA System using Multiple Reasoning Paths
Source: arXiv:2005.10970 source file (2020-05-22)
Supplement: Supplementary file 1 [file appendix.tex]

\subsubsection{Entity Lookup}
We integrate information from knowledge base into the model by constructing a memory matrix to store knowledge base, similar to~\cite{DBLP:conf/emnlp/MillerFDKBW16}. Each memory slot is a key-value pair to denote a fact in the knowledge base, where the key $k=[\varepsilon(e_{head});\varepsilon(r_{mid})]$ is a vector representation which composed of the embeddings of head entity (subject) and the relation, and the value $v=\varepsilon(e_{tail})$ is a vector representation of the tail entity (object). Both relation and entity embeddings are pre-trained and not updated by our model. Similar to Key-value memory networks, our entity lookup module involves the following steps: 

(1) Key hashing and addressing: in our model, predicted relation $r$ can be seen as topic of the sub-question and used to pre-select a list of candidate $\mathcal{KB}$ facts. This operation can dramatically reduce the search space of the following matching process. It is done by filtering out memory slots where their keys do not contain $r$ ($\emph{i.e.}\ r_{mid}\neq r$). Each remaining memory slot is then assigned a relevance score $\beta$ by comparing its key with representations of previous entity and current relation: %$s_0$ is the embedding of the topic entity labeled by an entity linker tool.
\begin{align}
z_{tj} = b([s_{t-1};h_t], k_j)
\end{align}
\vspace{-3ex}
\begin{align}
\beta_{tj} = \frac{\exp (z_{tj})}{\sum_i\exp (z_{ti})}
\end{align}

where $b$ is a parameterized feed-forward neural network used to measure the similarity between two inputs. 
% $\beta$ is a normalized score to represent relevance.

(2) Value reading: the values of memories are read by taking their weighted sum using the relevance scores.
\begin{align}
s_t =\sum_{i}\beta_{ti}v_i
\end{align}

The entity lookup step can be seen as executing a query in embedding space. The model use a head entity and a relation to search for the object from the memory, and the output $s$ can be seen as the representation of the searching result. 

\subsubsection{Answer prediction} The model stops making any predictions until it predicts a special relation \textit{$\textless$eop$\textgreater$}, which denotes the end of the path. We define the last tail entity output by entity lookup module as the final answer, and accordingly the probability of predicting the $i$-th entity in the memory as the answer:
\begin{align}
g_i = \beta_{(T-1)i}
\label{eq:e_prob}
\end{align}

where $T$ is the final timestep that outputs the \textit{$\textless$eop$\textgreater$} relation. The alternative way to predict the answer would be passing $s_t$ to another \textit{Softmax} layer and use the output normalized score as answer probability. However, it dramatically increases the training difficulty by introducing new training parameters. Also, this prediction method can only output the top one entity from the ranked probabilities list, while lose the ability to predict multiple qualified answers during inference.

The model then concatenates temporary hidden state $h_{t}'$, entity representation $\varepsilon(e_{t-1})$, and question context $c_t$ together, and pass the concatenation through an gating function $g(\cdot)$. This gating mechanism equips the model with ability to assign different wights on different features. At last, the model has a \textit{Softmax} output layer to generate probabilities to each candidate relation.  The process can be formally described by the following equations:
\begin{align}
[z_t^{h'}, z_t^{e}, z_t^{c}] = g([h'_{t}; \varepsilon(e_{t-1}); c_t])
\end{align}
\vspace{-2ex}
\begin{align}
h_{t} = \phi(z^{h'}_tW^{h'}h'_{t}+z^{e}_t W^{e}\varepsilon(e_{t-1})+z^{c}_t W^{c}c_{t})
\end{align}
\vspace{-2ex}
\begin{align}
o^j_t = \frac{\exp <h_t,\varepsilon(r_j)>}{\sum_k\exp <h_t,\varepsilon(r_k)>}
\label{eq:r_prob}
\end{align}

where $\phi$ represents one layer neural network with ReLU activation, $W^{(*)}$ are parameter matrices, $\varepsilon$ is the embedding gathering function, $<>$ outputs the dot product between two inputs, and $o_t^j$ is the probability of predicting the $j$-th relation in $\mathcal{R}$ at timestep $t$. After the model predicts a relation $r_t$, it can simply execute a query $(e_{t-1}, r_{t-1}, ?e_t)$ to get an entity $e_t$ from the knowledge base. The other way to collect this entity is via a soft lookup with a key-value memory network structure. We provide more details in the appendix.

At a timestep $t$, previous relations and entities consist the current reasoning path $\mathbf{r_t} = (e_{0},r_{1},e_{1},r_{2}, \cdots,e_{t-1})$. Our model take input features from three sources: question context $c$, previous entity $e$, and path history $h'$. The probability of predicting the relation $r_t$ can be written using these notations as follows:

\begin{equation}
\begin{aligned}
P(r_t|q,\mathbf{r_t}) = P(r_t|c_t, e_{t-1}, h'_t) \\
       = \sum_{f_t \in (c_t,e_t,h'_t)}P(z_t^f|c_t,e_{t-1},h'_t)P(r_t|f_t)
\end{aligned}
\end{equation}
